# Supplementary material for: Efficient Online Learning with Memory via Frank-Wolfe Optimization: Algorithms with Bounded Dynamic Regret and Applications to Control
Source: arXiv:2301.00497 source file (2023-03-31)
Supplement: Supplementary file 4 [file Appendix-Experiments.tex]

\section{Supplementary for Experiments}

% \begin{figure}[t!]
%     \captionsetup{font=footnotesize}
% 	\centering
% 	\vspace{1mm}
% 	\includegraphics[width=0.45\textwidth]{LaTeX/Text/Fig/CumLoss-slow.pdf}
% 	\caption{{Cumulative loss with sinusoidal weights in \cref{eq_loss_1}.}}
% 	\label{fig_CumLoss_slow}
% \end{figure} 

% \begin{figure}[t!]
%     \captionsetup{font=footnotesize}
% 	\centering
% 	\vspace{1mm}
% 	\includegraphics[width=0.45\textwidth]{LaTeX/Text/Fig/CumLoss-abrupt.pdf}
% 	\caption{{Cumulative loss with step weights in \cref{eq_loss_2}.}}
% 	\label{fig_CumLoss_abrupt}
% \end{figure} 

\begin{figure}[f]
    \centering
    \subfigure[Cumulative loss with sinusoidal weights in \cref{eq_loss_1}.]{\includegraphics[width=0.49\textwidth]{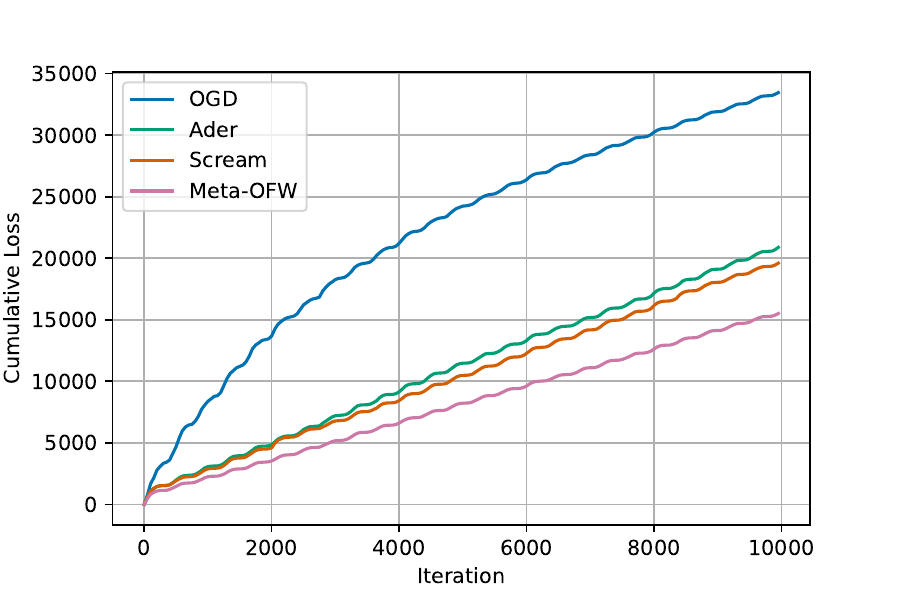}\label{fig_CumLoss_Gaussian_slow}}
    \subfigure[Cumulative loss with step weights in \cref{eq_loss_2}..]{\includegraphics[width=0.49\textwidth]{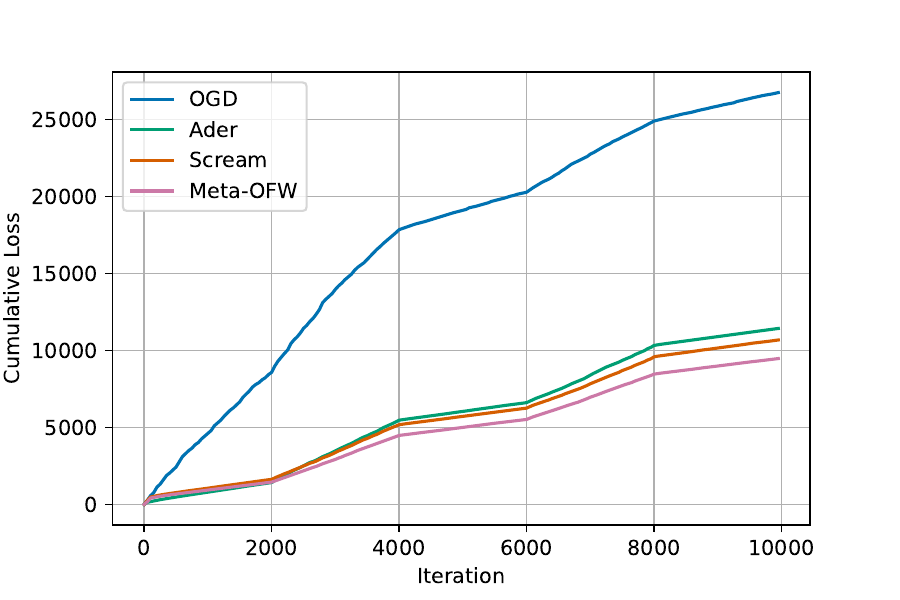}\label{fig_CumLoss_Gaussian_abrupt}}
    \caption{Cumulative loss with Gaussian distribution.}
    \label{fig_CumLoss_Gaussian}
\end{figure}
