# Supplementary material for: Efficient Online Learning with Memory via Frank-Wolfe Optimization: Algorithms with Bounded Dynamic Regret and Applications to Control
Source: arXiv:2301.00497 source file (2023-03-31)
Supplement: Supplementary file 9 [file Appendix-OFW-old.tex]

\section{Dynamic Regret of Frank-Wolf Algorithm with Memoryless Loss Function}\label{app:OFW_Memoryless}

\subsection{Proof of \Cref{theorem:OFW_Memoryless}}
To prove \Cref{theorem:OFW_Memoryless}, we take summation on both sides from $t=1$ to $T$ of \cref{eq:lemma_OFW_Memoryless} in \cref{lemma:OFW_Memoryless}, we get
\begin{equation}
	\begin{aligned}
		\sum_{t=1}^{T} \left(f_{t} \left(\mathbf{x}_{t}\right)-f_{t}\left(\mathbf{v}_{t}\right)\right) \leq & \sum_{t=1}^{T} \left(f_{t, t-1}^{\sup }+f_{t-1}\left(\mathbf{v}_{t-1}\right)-f_{t}\left(\mathbf{v}_{t}\right) \right)\\
		& +(1-\gamma)\left(\sum_{t=1}^{T-1}\left(f_{t}\left(\mathbf{x}_{t}\right)-f_{t}\left(\mathbf{v}_{t}\right)\right)+f_{0}\left(\mathbf{x}_{0}\right)-f_{0}\left(\mathbf{v}_{0}\right)\right) \\
		& +\gamma D \sum_{t=1}^{T}\left\|\nabla f_{t}\left(\mathbf{x}_{t}\right)-\nabla f_{t-1}\left(\mathbf{x}_{t-1}\right)\right\|+\gamma^{2} T \frac{3 L_{1} D^{2}}{2}
	\end{aligned}
\label{eq:theorem_OFW_Memoryless_1}
\end{equation}
where $f_{t, t-1}^{\text {sup }}$ is defined in \Cref{lemma:OFW_Memoryless}. Moving $(1-\gamma) \sum_{t=1}^{T-1}\left(f_{t}\left(\mathbf{x}_{t}\right)-f_{t}\left(\mathbf{v}_{t}\right) \right)$ to the left side of \cref{eq:theorem_OFW_Memoryless_1}, and noting $\sum_{t=1}^{T}\left( f_{t-1}\left(\mathbf{v}_{t-1}\right)- f_{t}\left(\mathbf{v}_{t}\right)\right)=$ $f_{0}\left(\mathbf{v}_{0}\right)-f_{T}\left(\mathbf{v}_{T}\right)$, we get
\begin{equation}
	\begin{aligned}
	\gamma \sum_{t=1}^{T-1}\left(f_{t}\left(\mathbf{x}_{t}\right)-f_{t}\left(\mathbf{v}_{t}\right)\right)+\left(f_{T}\left(\mathbf{x}_{T}\right)-f_{T}\left(\mathbf{v}_{T}\right)\right) \leq & \sum_{t=1}^{T} f_{t, t-1}^{\mathrm{sup}}+(1-\gamma)\left(f_{0}\left(\mathbf{x}_{0}\right)-f_{0}\left(\mathbf{v}_{0}\right)\right)+f_{0}\left(\mathbf{v}_{0}\right)-f_{T}\left(\mathbf{v}_{T}\right) \\
	&+\gamma D \sum_{t=1}^{T}\left\|\nabla f_{t}\left(\mathbf{x}_{t}\right)-\nabla f_{t-1}\left(\mathbf{x}_{t-1}\right)\right\|+\gamma^{2} T \frac{3 L_{1} D^{2}}{2}
	\end{aligned}
\label{eq:theorem_OFW_Memoryless_2}
\end{equation}

Since $\gamma<1$, the left hand side of \cref{eq:theorem_OFW_Memoryless_2} is lower bounded by $\gamma \sum_{t=1}^{T}\left(f_{t}\left(\mathbf{x}_{t}\right)-f_{t}\left(\mathbf{v}_{t}\right)\right)$. Since $(1-\gamma)<1$, we can write \cref{eq:theorem_OFW_Memoryless_2} as
\begin{equation}
	\gamma \DyReg \leq  \sum_{t=1}^{T} f_{t, t-1}^{\sup }+\left(f_{0}\left(\mathbf{x}_{0}\right)-f_{T}\left(\mathbf{v}_{T}\right)\right)+\gamma^{2} T \frac{3 L_{1} D^{2}}{2} +\gamma D \sum_{t=1}^{T}\left\|\nabla f_{t}\left(\mathbf{x}_{t}\right)-\nabla f_{t-1}\left(\mathbf{x}_{t-1}\right)\right\|
\label{eq:theorem_OFW_Memoryless_3}
\end{equation}

Divide both sides of \cref{eq:theorem_OFW_Memoryless_3} by $\gamma$ and substitute the following identity
\begin{equation}
	\sum_{t=1}^{T}\left\|\nabla f_{t}\left(\mathbf{x}_{t}\right)-\nabla f_{t-1}\left(\mathbf{x}_{t-1}\right)\right\| \leq \sqrt{T \sum_{t=1}^{T}\left\|\nabla f_{t}\left(\mathbf{x}_{t}\right)-\nabla f_{t-1}\left(\mathbf{x}_{t-1}\right)\right\|^{2}}=\sqrt{T D_{T}}
\label{eq:theorem_OFW_Memoryless_4}
\end{equation}

into \cref{eq:theorem_OFW_Memoryless_3} with the definition of $V_{T}$ to obtain
\begin{equation}
\DyReg \leq \frac{1}{\gamma} V_{T}+\frac{1}{\gamma}\left(f_{0}\left(\mathbf{x}_{0}\right)-f_{T}\left(\mathbf{v}_{T}\right) \right) + D \sqrt{T D_{T}}+\gamma T \frac{3 L_{1} D^{2}}{2}
\label{eq:theorem_OFW_Memoryless_5}
\end{equation}

Select $\gamma=\calO(\frac{1}{\sqrt{T}})$ and use $(1-\gamma)<1$ to write
\begin{equation}
\DyReg \leq \cal{O}\left(\text{$\sqrt{T}$}\left(\text{$1+V_{T}$}+\text{$\sqrt{D_{T}}$}\right)\right).
\label{eq:theorem_OFW_Memoryless_6}
\end{equation} \qed



\subsection{Proof of \Cref{lemma:OFW_Memoryless}}

\begin{lemma}\label{lemma:OFW_Memoryless}
	Under \Cref{assumption:bounded_set} and \Cref{assumption:smooth_loss}, \Cref{alg:OFW_Memoryless} satisfies the following descent relations,
	\begin{equation}
    	\begin{aligned}
        	f_{t}\left(\mathbf{x}_{t}\right)-f_{t}\left(\mathbf{v}_{t}\right) \leq & f_{t, t-1}^{\text {sup }}+(1-\gamma)\left(f_{t-1}\left(\mathbf{x}_{t-1}\right)-f_{t-1}\left(\mathbf{v}_{t-1}\right)\right) \\
        	&+f_{t-1}\left(\mathbf{v}_{t-1}\right)-f_{t}\left(\mathbf{v}_{t}\right)+\gamma^{2} \frac{3 L_{1}}{2} D^{2} \\
        	&+\gamma D\left\|\nabla f_{t}\left(\mathbf{x}_{t}\right)-\nabla f_{t-1}\left(\mathbf{x}_{t-1}\right)\right\|
    	\end{aligned}
    	\label{eq:lemma_OFW_Memoryless}
	\end{equation}
	where $f_{t, t-1}^{\text {sup}}\triangleq\sup _{\mathbf{x} \in \mathcal{X}}\left|f_{t}(\mathbf{x})-f_{t-1}(\mathbf{x})\right|$ is the instantaneous maximum cost variation.
\end{lemma}

\begin{proof}
By \cref{assumption:smooth_loss}, we have
	\begin{equation}
    	f_{t}\left(\mathbf{x}_{t}\right) \leq  f_{t}\left(\mathbf{x}_{t-1}\right)+\left\langle\nabla f_{t}\left(\mathbf{x}_{t-1}\right), \mathbf{x}_{t}-\mathbf{x}_{t-1}\right\rangle+\frac{L_{1}}{2}\left\|\mathbf{x}_{t}-\mathbf{x}_{t-1}\right\|^{2}.
    	\label{eq:lemma_OFW_Memoryless_1}
	\end{equation}
	
Substituting the update for $\mathbf{x}_t$ in \Cref{alg:OFW_Memoryless}, \ie $\left(\mathbf{x}_{t}-\mathbf{x}_{t-1}\right)=\gamma\left(\mathbf{x}_{t-1}^\prime-\mathbf{x}_{t-1}\right)$, into \cref{eq:lemma_OFW_Memoryless_1},
	\begin{equation}
    	f_{t}\left(\mathbf{x}_{t}\right) \leq  f_{t}\left(\mathbf{x}_{t-1}\right)+\gamma\left\langle\nabla f_{t}\left(\mathbf{x}_{t-1}\right), \mathbf{x}_{t-1}^\prime-\mathbf{x}_{t-1}\right\rangle +\gamma^{2} \frac{L_{1}}{2}\left\|\mathbf{x}_{t-1}^\prime-\mathbf{x}_{t-1}\right\|^{2} .
    	\label{eq:lemma_OFW_Memoryless_2}
	\end{equation}
	
Adding and subtracting the terms $\gamma\left\langle\nabla f_{t-1}\left(\mathbf{x}_{t-1}\right), \mathbf{x}_{t-1}^\prime-\right.$ $\left.\mathbf{x}_{t-1}\right\rangle$ to the right hand side of \cref{eq:lemma_OFW_Memoryless_2}, we obtain
	\begin{equation}
    	\begin{aligned}
        	f_{t}\left(\mathbf{x}_{t}\right) \leq & f_{t}\left(\mathbf{x}_{t-1}\right)+\gamma\left\langle\nabla f_{t}\left(\mathbf{x}_{t-1}\right)-\nabla f_{t-1}\left(\mathbf{x}_{t-1}\right), \mathbf{x}_{t-1}^\prime-\mathbf{x}_{t-1}\right\rangle \\
        	&+\gamma\left\langle\nabla f_{t-1}\left(\mathbf{x}_{t-1}\right), \mathbf{x}_{t-1}^\prime-\mathbf{x}_{t-1}\right\rangle +\gamma^{2} \frac{L_{1}}{2}\left\|\mathbf{x}_{t-1}^\prime-\mathbf{x}_{t-1}\right\|^{2}.
        	\end{aligned}
    	\label{eq:lemma_OFW_Memoryless_3}
	\end{equation}
	
Next, noting the optimality condition of $\mathbf{x}_{t-1}^\prime$, \ie
	\begin{equation}
    	\left\langle\mathbf{v}_{t-1}, \nabla f_{t-1}\left(\mathbf{x}_{t-1}\right)\right\rangle  \geq \min _{\mathbf{x} \in \mathcal{X}}\left\langle\mathbf{x}, \nabla f_{t-1}\left(\mathbf{x}_{t-1}\right)\right\rangle =\left\langle\mathbf{x}_{t-1}^\prime, \nabla f_{t-1}\left(\mathbf{x}_{t-1}\right)\right\rangle,
	    \label{eq:lemma_OFW_Memoryless_4}
	\end{equation}
and substituting into \cref{eq:lemma_OFW_Memoryless_3} leads to
	\begin{equation}
    	\begin{aligned}
        	f_{t}\left(\mathbf{x}_{t}\right) \leq & f_{t}\left(\mathbf{x}_{t-1}\right)+\gamma\left\langle\nabla f_{t}\left(\mathbf{x}_{t-1}\right)-\nabla f_{t-1}\left(\mathbf{x}_{t-1}\right), \mathbf{x}_{t-1}^\prime-\mathbf{x}_{t-1}\right\rangle \\
        	&+\gamma\left\langle\nabla f_{t-1}\left(\mathbf{x}_{t-1}\right), \mathbf{v}_{t-1}-\mathbf{x}_{t-1}\right\rangle +\gamma^{2} \frac{L_{1}}{2}\left\|\mathbf{x}_{t-1}^\prime-\mathbf{x}_{t-1}\right\|^{2}
    	\end{aligned}
    	\label{eq:lemma_OFW_Memoryless_5}
	\end{equation}
	
By convexity of of $f_{t-1}(\cdot)$ in \cref{eq:lemma_OFW_Memoryless_5}, we have
	\begin{equation}
    	\begin{aligned}
        	f_{t}\left(\mathbf{x}_{t}\right) \leq & f_{t}\left(\mathbf{x}_{t-1}\right)+\gamma\left\langle\nabla f_{t}\left(\mathbf{x}_{t-1}\right)-\nabla f_{t-1}\left(\mathbf{x}_{t-1}\right), \mathbf{x}_{t-1}^\prime-\mathbf{x}_{t-1}\right\rangle \\
        	&+\gamma\left(f_{t-1}\left(\mathbf{v}_{t-1}\right)-f_{t-1}\left(\mathbf{x}_{t-1}\right)\right) +\gamma^{2} \frac{L_{1}}{2}\left\|\mathbf{x}_{t-1}^\prime-\mathbf{x}_{t-1}\right\|^{2}
    	\end{aligned}
    	\label{eq:lemma_OFW_Memoryless_6}
	\end{equation}
	
	Subtracting $f_{t}\left(\mathbf{v}_{t}\right)$ from both sides of \cref{eq:lemma_OFW_Memoryless_6} gives
	\begin{equation}
	\begin{aligned}
	f_{t}\left(\mathbf{x}_{t}\right)-f_{t}\left(\mathbf{v}_{t}\right) \leq & f_{t}\left(\mathbf{x}_{t-1}\right)-f_{t}\left(\mathbf{v}_{t}\right) + \gamma\left\langle\nabla f_{t}\left(\mathbf{x}_{t-1}\right)-\nabla f_{t-1}\left(\mathbf{x}_{t-1}\right), \mathbf{x}_{t-1}^\prime-\mathbf{x}_{t-1}\right\rangle \\
	&+\gamma\left(f_{t-1}\left(\mathbf{v}_{t-1}\right)-f_{t-1}\left(\mathbf{x}_{t-1}\right)\right) +\gamma^{2} \frac{L_{1}}{2}\left\|\mathbf{x}_{t-1}^\prime-\mathbf{x}_{t-1}\right\|^{2} .
	\end{aligned}
	\label{eq:lemma_OFW_Memoryless_7}
	\end{equation}
	
Next, consider the term $f_{t}\left(\mathbf{x}_{t-1}\right)-f_{t}\left(\mathbf{v}_{t}\right)$ from the right hand side of \cref{eq:lemma_OFW_Memoryless_7}. We can bound it as follows,
	\begin{equation}
    	\begin{aligned}
    	    f_{t}\left(\mathbf{x}_{t-1}\right)-f_{t}\left(\mathbf{v}_{t}\right)&=f_{t}\left(\mathbf{x}_{t-1}\right)-f_{t-1}\left(\mathbf{x}_{t-1}\right)+f_{t-1}\left(\mathbf{x}_{t-1}\right)-f_{t-1}\left(\mathbf{v}_{t-1}\right)+f_{t-1}\left(\mathbf{v}_{t-1}\right)-f_{t}\left(\mathbf{v}_{t}\right) \\
    	    &\leq  f_{t, t-1}^{\text {sup }}+f_{t-1}\left(\mathbf{x}_{t-1}\right)-f_{t-1}\left(\mathbf{v}_{t-1}\right) +f_{t-1}\left(\mathbf{v}_{t-1}\right)-f_{t}\left(\mathbf{v}_{t}\right),
    	\end{aligned}
	\label{eq:lemma_OFW_Memoryless_8}
	\end{equation}
% Bounding the $f_{t}\left(\mathbf{x}_{t-1}\right)-f_{t-1}\left(\mathbf{x}_{t-1}\right)$ by its absolute value, and then taking the supremum over $\mathbf{x} \in \mathcal{X}$, we get
% 	\begin{equation}
% 	f_{t}\left(\mathbf{x}_{t-1}\right)-f_{t}\left(\mathbf{v}_{t}\right) \leq  f_{t, t-1}^{\text {sup }}+f_{t-1}\left(\mathbf{x}_{t-1}\right)-f_{t-1}\left(\mathbf{v}_{t-1}\right) +f_{t-1}\left(\mathbf{v}_{t-1}\right)-f_{t}\left(\mathbf{v}_{t}\right)
% 	\label{eq:lemma_OFW_Memoryless_9}
% 	\end{equation}
where $f_{t, t-1}^{\text {sup }}\triangleq\sup _{\mathbf{x} \in \mathcal{X}}\left|f_{t}(\mathbf{x})-f_{t-1}(\mathbf{x})\right|$. Substituting \cref{eq:lemma_OFW_Memoryless_8} into \cref{eq:lemma_OFW_Memoryless_7}, we obtain
	\begin{equation}
	\begin{aligned}
	f_{t}\left(\mathbf{x}_{t}\right)- f_{t}\left(\mathbf{v}_{t}\right) \leq & f_{t, t-1}^{\text {sup }}+(1-\gamma)\left(f_{t-1}\left(\mathbf{x}_{t-1}\right)-f_{t-1}\left(\mathbf{v}_{t-1}\right)\right)+f_{t-1}\left(\mathbf{v}_{t-1}\right)-f_{t}\left(\mathbf{v}_{t}\right) \\
	&+\gamma\left\langle\nabla f_{t}\left(\mathbf{x}_{t-1}\right)-\nabla f_{t-1}\left(\mathbf{x}_{t-1}\right), \mathbf{x}_{t-1}^\prime-\mathbf{x}_{t-1}\right\rangle +\gamma^{2} \frac{L_{1}}{2}\left\|\mathbf{x}_{t-1}^\prime-\mathbf{x}_{t-1}\right\|^{2}
	\end{aligned}
	\label{eq:lemma_OFW_Memoryless_9}
	\end{equation}
	
Further, the inner product term in \cref{eq:lemma_OFW_Memoryless_9} can be written as
	\begin{equation}
    	\left\langle\nabla f_{t}\left(\mathbf{x}_{t-1}\right)-\nabla f_{t-1}\left(\mathbf{x}_{t-1}\right), \mathbf{x}_{t-1}^\prime-\mathbf{x}_{t-1}\right\rangle =\left\langle\nabla f_{t}\left(\mathbf{x}_{t-1}\right)-\nabla f_{t}\left(\mathbf{x}_{t}\right)+\nabla f_{t}\left(\mathbf{x}_{t}\right)-\nabla f_{t-1}\left(\mathbf{x}_{t-1}\right), \mathbf{x}_{t-1}^\prime-\mathbf{x}_{t-1}\right\rangle
    	\label{eq:lemma_OFW_Memoryless_10}
	\end{equation}
	
Substituting \cref{eq:lemma_OFW_Memoryless_10} into \cref{eq:lemma_OFW_Memoryless_9} and applying the Cauchy-Schwartz inequality, we get
	\begin{equation}
	\begin{aligned}
	f_{t}\left(\mathbf{x}_{t}\right)-f_{t}\left(\mathbf{v}_{t}\right) 
	\leq & f_{t, t-1}^{\text {sup }}+(1-\gamma)\left(f_{t-1}\left(\mathbf{x}_{t-1}\right)-f_{t-1}\left(\mathbf{v}_{t-1}\right)\right)+f_{t-1}\left(\mathbf{v}_{t-1}\right)-f_{t}\left(\mathbf{v}_{t}\right) \\
	&+\gamma\left\|\nabla f_{t}\left(\mathbf{x}_{t-1}\right)-\nabla f_{t}\left(\mathbf{x}_{t}\right)\right\|\left\|\mathbf{x}_{t-1}^\prime-\mathbf{x}_{t-1}\right\|+\gamma\left\|\nabla f_{t}\left(\mathbf{x}_{t}\right)-\nabla f_{t-1}\left(\mathbf{x}_{t-1}\right)\right\|\left\|\mathbf{x}_{t-1}^\prime-\mathbf{x}_{t-1}\right\| \\
	&+\gamma^{2} \frac{L_{1}}{2}\left\|\mathbf{x}_{t-1}^\prime-\mathbf{x}_{t-1}\right\|^{2}
	\end{aligned}
	\label{eq:lemma_OFW_Memoryless_12}
	\end{equation}
	
	Using \Cref{assumption:smooth_loss} and the update for $\mathbf{x}_{t}$, we get
	\begin{equation}
	\begin{aligned}
	f_{t}\left(\mathbf{x}_{t}\right)-f_{t}\left(\mathbf{v}_{t}\right) \leq & f_{t, t-1}^{\text {sup }}+(1-\gamma)\left(f_{t-1}\left(\mathbf{x}_{t-1}\right)-f_{t-1}\left(\mathbf{v}_{t-1}\right)\right) \\
	&+f_{t-1}\left(\mathbf{v}_{t-1}\right)-f_{t}\left(\mathbf{v}_{t}\right)+\gamma^{2} \frac{3 L_{1}}{2}\left\|\mathbf{x}_{t-1}^\prime-\mathbf{x}_{t-1}\right\|^{2} \\
	&+\gamma\left\|\nabla f_{t}\left(\mathbf{x}_{t}\right)-\nabla f_{t-1}\left(\mathbf{x}_{t-1}\right)\right\|\left\|\mathbf{x}_{t-1}^\prime-\mathbf{x}_{t-1}\right\| .
	\end{aligned}
	\label{eq:lemma_OFW_Memoryless_13}
	\end{equation}	
	
	Utilizing \Cref{assumption:bounded_set} provides the result in \Cref{lemma:OFW_Memoryless}.
\end{proof}
